# Supplementary material for: A General Decoupled Learning Framework for Parameterized Image Operators
Source: arXiv:1907.05852 source file (2019-07-11)
Supplement: Supplementary file 1 [file eccv_figure2_supp.tex]

\begin{figure*}[t]
\begin{center}
\begin{tabular}{c}
\includegraphics[width=6cm]{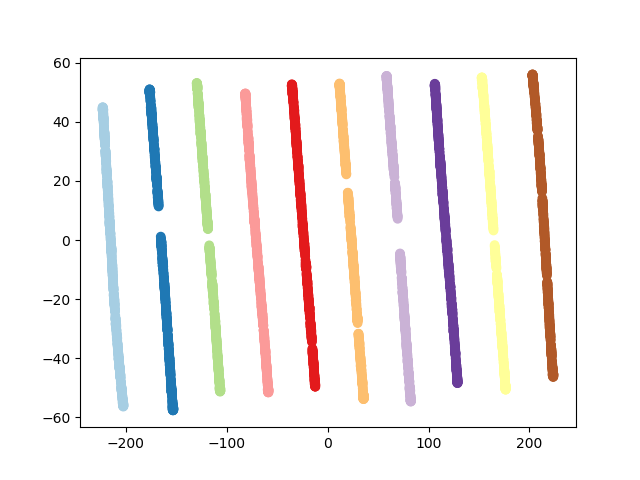}
\end{tabular}
\end{center}

\caption{T-SNE illustration of the learned weights of the 2nd convolution layer in the base network. The displayed convolution weights are generated by the jointly trained network with 10 image operators. Each color indicates one specific operator. We also observe similar visualized results for the other convolution layers.}

\label{figure:eecv_2_supp}
\end{figure*}
